# Supplementary material for: Non-Hermitian extensions of higher-order topological phases and their biorthogonal bulk-boundary correspondence
Source: arXiv:1812.09060 ancillary file (2019-03-06)
Supplement: Supplementary file 1 [file NHhigherorderSupMat-resubmitPRB.pdf]

# Supplementary Material for Non-Hermitian extensions of higher-order topological phases and their biorthogonal bulk-boundary correspondence

Elisabet Edvardsson, Flore K. Kunst, and Emil J. Bergholtz
*Department of Physics, Stockholm University, AlbaNova University Center, 106 91 Stockholm, Sweden*
(Dated: February 1, 2019)

In this supplementary material we give the Bloch-Hamiltonian for the non-Hermitian chiral hinge insulator and include the real and imaginary part of the spectrum of all of the three explicit models discussed in the main text, as well as plots of the eigenvalue spectrum in the complex plane for the breathing kagome in the rhombus geometry. We additionally include density plots for several bands for the breathing kagome in the rhombus and triangle geometries.

*Bloch-Hamiltonian for the hinge state model.*— The Bloch-Hamiltonian for the hinge state model in the basis $\left\{c_A^\dagger\left|0\right\rangle, c_{B'}^\dagger\left|0\right\rangle, c_{B''}^\dagger\left|0\right\rangle, c_B^\dagger\left|0\right\rangle\right\}$ is given by

$$H = \begin{pmatrix} -\sin(t) & s(1+\mathrm{e}^{-\mathrm{i}k_y}) & 0 & a_+(t)+b(t)\mathrm{e}^{-\mathrm{i}k_x} \\ s(1+\mathrm{e}^{\mathrm{i}k_y}) & \sin(t) & a_+(t)+b(t)\mathrm{e}^{-\mathrm{i}k_x} & 0 \\ 0 & a_-(t)+b(t)\mathrm{e}^{\mathrm{i}k_x} & -\sin(t) & s(1+\mathrm{e}^{-\mathrm{i}k_y}) \\ a_-(t)+b(t)\mathrm{e}^{\mathrm{i}k_x} & 0 & s(1+\mathrm{e}^{\mathrm{i}k_y}) & \sin(t) \end{pmatrix}, \tag{1}$$

with $a_\pm(t)$ and $b(t)$ defined as in the main text.

*Real and imaginary energies.*— In Fig. 1, we show the real (top) and imaginary (bottom) part of the spectrum for the hinge state model (Fig. 1(a)) and the breathing kagome model in the geometry of a rhombus (Fig. 1(b)) and triangle (Fig. 1(c)) of which the absolute value of the spectrum is shown in Figs. 1(b), 3(b) and 4(b), respectively, in the main text.

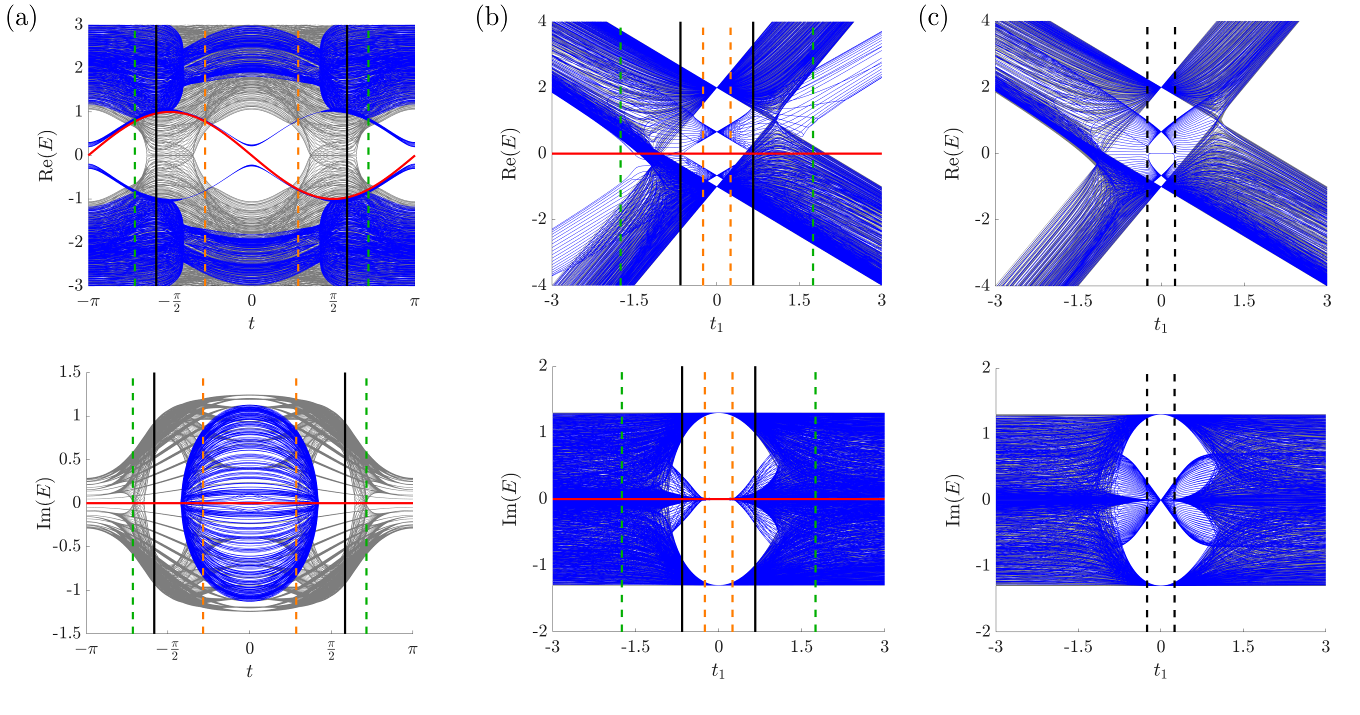


FIG. 1: Real (top) and imaginary (bottom) part of the energy spectrum of (a) the hinge state model in Fig. 1 in the main text, and the breathing kagome model in (b) the rhombus and (c) triangle geometries in Figs. 3 and 4, respectively, in the main text with the same choice of parameters. Gray and blue lines correspond to the spectra of the periodic and open systems respectively. The orange (green) dashed lines in (a) and (b) correspond to $|r_{R,1}| = |r_{L,2}| = 1$ ($|r_{R,2}| = |r_{L,1}| = 1$), while the black solid lines correspond to $|r_{L,1}r_{R,1}| = |r_{L,2}r_{R,2}| = 1$, and the red lines correspond to the hinge and corner states in (a) and (b) respectively. The black dashed lines in (c) correspond to $|r_{R,2}| = |r_{L,1}| = 1$.

In Fig. 2, we show plots of the eigenvalue spectrum for the breathing kagome lattice in the rhombus geometry on

the complex plane with the same choice of parameter values as in the main text for different values of $t_1$. We see that the gap is closed at $|r_{L,1}r_{R,1}| = |r_{L,2}r_{R,2}| = 1$, where $t_1 = \sqrt{7}/4 \approx 0.66144$.

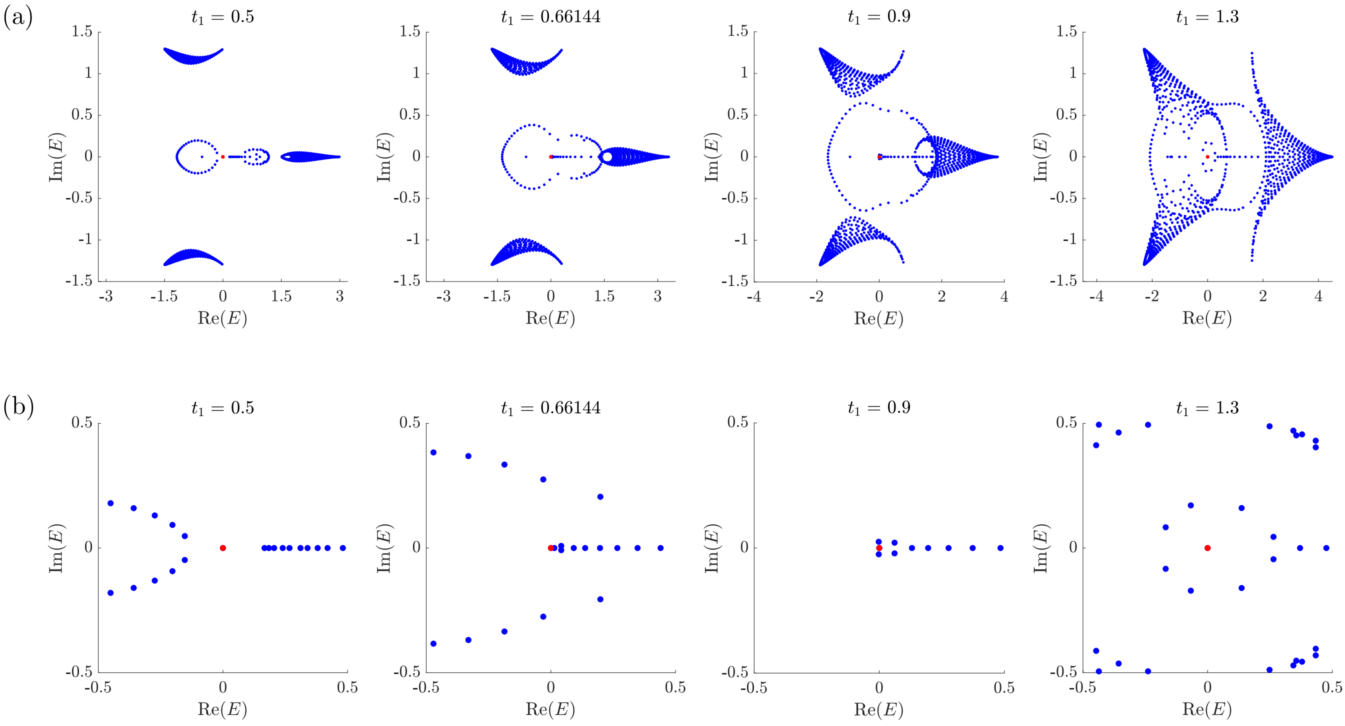


FIG. 2: Eigenvalue spectrum for the breathing kagome lattice in the rhombus geometry with the same parameter values as in the main text for some values of $t_1$ in the complex plane. The corner state with $E = 0$ is marked in red. In (a) all eigenvalues are shown, while in (b) we zoom in around the corner state.

*Distribution of states in breathing kagome lattice in rhombus geometry.*— In Fig. 3, we show the wave function distribution, i.e., $\langle \Pi_{m_1,m_2} \rangle^n_{\alpha\alpha'}$ with $\alpha, \alpha' \in \{R, L\}$, of several energy bands in the spectrum of the breathing kagome lattice in the rhombus geometry computed for $|r_{L,1}r_{R,1}| = |r_{L,2}r_{R,2}| = 1$. We see that the blue bands to which the zero-energy corner state (in red in Fig. 3(b) in the main text, and in Fig. 1(b)) attaches, i.e., $|E| = 0.28875$ and $|E| = 0.97022$, are corner and edge states in the language of right and left wave functions, but behave as bulk states when considered from the perspective of the biorthogonal localization.

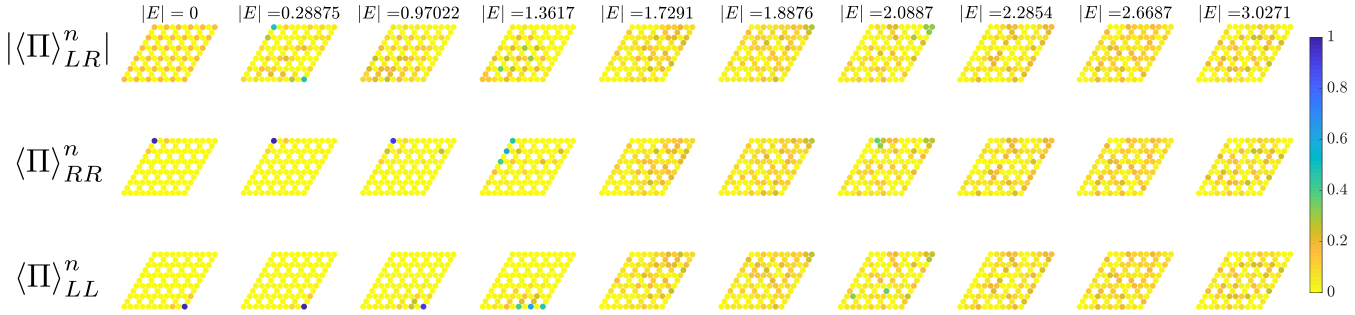


FIG. 3: Localization of the energy band explicitly indicated on a breathing kagome lattice in the geometry of a rhombus with $M_1 = M_2 = 6$ using the biorthogonal (top), right (middle) and left (bottom) expectation value of the projection operator for $t_1 = 0.66$, $t_2 = 1$ and $\gamma = 1.5$.

*Distribution of states in breathing kagome lattice in triangle geometry.*— In Fig. 4, we show the wave function distribution, i.e., $\langle \Pi_{m_1,m_2} \rangle^n_{\alpha\alpha'}$ with $\alpha, \alpha' \in \{R, L\}$, of several energy bands in the spectrum of the breathing kagome lattice in the triangle geometry. We see that the biorthogonal localization reveals the same behavior as that of the right and left wave functions.

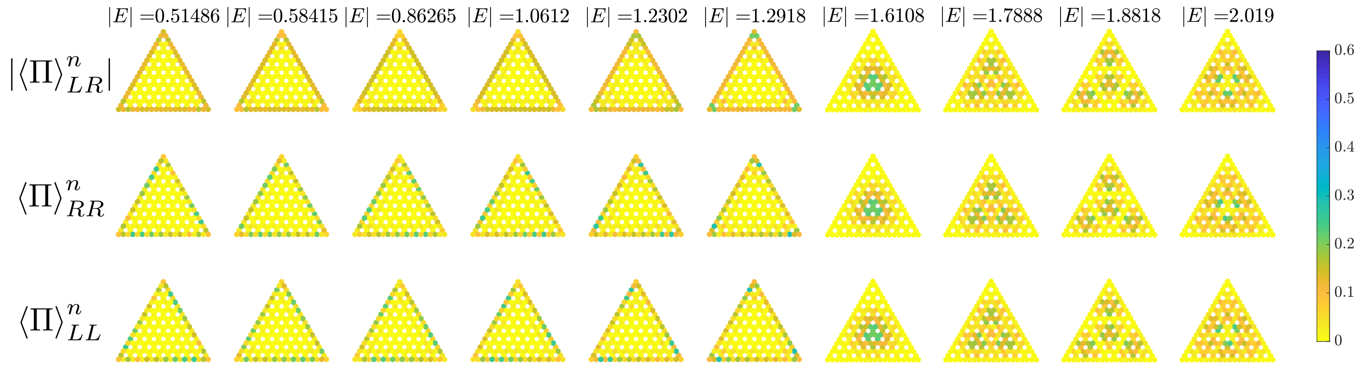


FIG. 4: Localization of the energy band explicitly indicated on a breathing kagome lattice in the geometry of a triangle with $M_1 = M_2 = 6$ using the biorthogonal (top), right (middle) and left (bottom) expectation value of the projection operator for $t_1 = 0.5$, $t_2 = 1$ and $\gamma = 1.5$.
